# Supplementary material for: From Imitation to Exploration: End-to-end Autonomous Driving based on World Model
Source: arXiv:2410.02253 source file (2025-04-20)
Supplement: Supplementary file 1 [file appendix-comparison.tex]

\section{Selection of Baselines} \label{appendix: select-baselines}

This section explains the reasons for selecting the following methods in the performance comparison experiments.

\subsection{Experts}

Due to the difficulty of the routes in CARLA's leaderboards, most end-to-end driving models cannot guarantee the completion of all the routes without relying on privileged information, such as the ground-truth states of surrounding traffic participants, precise positions of static obstacles, and the specific details of traffic signs. To estimate the upper limit performance of learning-based end-to-end driving models, we adapted several representative experts.

\subsubsection{Roach}

The RL-based expert developed by \cite{zhang2021end} serves as the coach that guides the training of the IL agent using only permissible data. This model leverages the states of traffic lights and semantic segmentation images as privileged information, effectively demonstrating RL's capability to formulate driving policies from scratch. We reproduced the performance of Roach's expert model on CARLA Leaderboard 1.0, and then adapted and trained it on CARLA Leaderboard 2.0. This approach allows us to illustrate the potential upper limits of model-free RL's performance in autonomous driving scenarios.

\subsection{Baselines}

We have reproduced various SOTA driving models on CARLA Leaderboard 1.0 and transited them to Leaderboard 2.0 to assess their ability of generalization. Notably, all the end-to-end driving models achieving top positions on the leaderboards are based on IL. IL possesses an advantage over model-free RL in its superior capacity to handle high-dimensional environmental data. Additionally, the availability of ground truth trajectory data facilitates faster convergence in the policy network. The absence of standout RL-based state-of-the-art models is another reason why we introduce RL-based expert models for comparison experiments.

\subsubsection{LAV}

LAV processes multi-modal sensory data, including RGB camera and LiDAR inputs, to directly output control commands \cite{chen2022learning}. The model is elegantly designed, emphasizing that the quality of the ground truth trajectory during training significantly influences performance. This model was selected because it ranks 1st regarding route completion rate on CARLA Leaderboard 1.0.

\subsubsection{Transfuser++}

Transfuser++ (TF++) is an enhanced version of Transfuser \cite{chitta2022transfuser, jaeger2023hidden}, maintaining a similar structure while improving the transformer's efficiency and reducing ambiguity in the model's output by disentangling trajectory prediction from velocity. Among the various implementations of Transfuser++, we opted to reproduce the version with waypoint prediction (TF++ WP) and adapted it for CARLA Leaderboard 2.0.

\subsubsection{TCP}

TCP is a camera-only IL model \cite{wu2022trajectory}, which proposes combining trajectory and control prediction outputs to enhance the model's generalization ability. This innovative framework allows TCP to be seamlessly integrated as an output module for other models. We have reproduced TCP's performance on CARLA Leaderboard 1.0 and transited it to Leaderboard 2.0 to evaluate its generalization ability.

\subsubsection{ReasonNet}

ReasonNet is the successor to InterFuser \cite{shao2023safety, shao2023reasonnet}. Its main improvement is the introduction of a global reasoning module that enhances the model's environmental understanding. This model has achieved the highest driving score on the CARLA Leaderboard 1.0. However, the code for ReasonNet has not been made public. Given that reproductions of InterFuser have shown a significant drop in performance\footnote{See \url{https://paperswithcode.com/sota/autonomous-driving-on-carla-leaderboard}.}, we cannot ensure the reproduction of ReasonNet would achieve similar results. Consequently, our comparison in Table \ref{table: performance-L10} is based  on the scores reported in the leaderboard.

% \subsubsection{CarLLaVA}

% CarLLaVA is an IL-based driving model that leverages a large language model LLaMA to encode the environmental context and imitate driving behavior generated by PDM-Lite \cite{renz2024carllava}. This model has achieved the highest driving score on the CARLA Leaderboard 2.0. The code for CarLLaVA has not been made public. Moreover, we cannot afford to train a model with the same scale as CarLLaVA due to a limit in computational resources. Therefore, our comparison in Table \ref{performance_comparison_20} is based on the scores reported in the leaderboard.
