# Supplementary material for: From Imitation to Exploration: End-to-end Autonomous Driving based on World Model
Source: arXiv:2410.02253 source file (2025-04-20)
Supplement: Supplementary file 2 [file appendix-leaderboard.tex]

\section{Analysis of CARLA's Leaderboard 2.0} \label{appendix: leaderboard-2}

To allow a higher efficiency in training process, we analysis the scenario types and their distributions in the routes provided in training, validation, and testing sets.

\subsection{Scenario Types}

According to the official statement, the scenarios in Carla Leaderboard 2.0 are randomly generated based on 10 scenario types referenced in \cite{najm2007pre}\footnote{See \url{https://leaderboard.carla.org/scenarios/}.}. However, in practice, there are a total of 38 distinct scenario types in annotation. By analyzing the actual behavior of these scenarios, we categorized them using a human-intuitive strategy. This approach groups similar scenarios together to facilitate more effective training of the behavior agent. The rough categorization is summarized in Table \ref{table: scenario-category}.

\begin{table}[htb]
     \centering
     \caption{Rough categorization of scenarios, sorted by difficulty}
     \label{table: scenario-category}
     \begin{tabular}{l|l|l}
      \toprule[2pt] \midrule
      \multirow{2}*{\parbox{1cm}{\textbf{Intuitive}\\\textbf{Strategy}}} & \multirow{2}*{\textbf{Scenario Type}} & \multirow{2}*{\textbf{Specialty}} \\
      & & \\ \midrule
      \multirow{3}*{Keeping} & InterurbanActorFlow \\
      & InterurbanAdvancedActorFlow \\
      & ControlLoss \\ \midrule
      \multirow{11}*{Yielding} & HardBreakRoute & \multirow{5}*{\parbox{2cm}{Threat from\\the front}} \\
      & ParkingCrossingPedestrian \\
      & PedestrianCrossing \\
      & DynamicObjectCrossing \\
      & CrossingBicycleFlow \\ \cmidrule{2-3}
      & HighwayCutIn & \multirow{6}*{\parbox{2cm}{Threat from\\the surrounding}} \\
      & ParkingCutIn \\
      & StaticCutIn \\
      & OppositeVehicleTakingPriority \\
      & OppositeVehicleRunningRedLight \\
      & YieldToEmergencyVehicle \\ \midrule
      \multirow{6}*{Entering} & HighwayExit & \multirow{6}*{Priority sensitive} \\
      & ParkingExit & \\
      & EnterActorFlow & \\
      & EnterActorFlowV2 & \\
      & MergerIntoSlowTraffic & \\
      & MergerIntoSlowTrafficV2 & \\ \midrule
      \multirow{9}*{Turning} & NonSignalizedJunctionRightTurn & Non-signalized; \\
      & NonSignalizedJunctionLeftTurn & priority sensitive \\ \cmidrule{2-3}
      & SignalizedJunctionRightTurn & Signalized; \\
      & SignalizedJunctionLeftTurn &  priority sensitive \\ \cmidrule{2-3}
      & PriorityAtJunction  & \multirow{5}*{Priority sensitive} \\
      & VehicleTurningRoutePedestrian & \\
      & VehicleTurningRoute & \\
      & BlockedIntersection & \\
      & InvadingTurn & \\ \midrule
      \multirow{9}*{Bypassing} & Accident & \multirow{4}*{\parbox{2cm}{Threat from\\the side}} \\
      & ConstructionObstacle & \\
      & HazardAtSideLane & \\
      & ParkedObstacle & \\ \cmidrule{2-3}
      & AccidentTwoWays & \multirow{5}*{\parbox{2cm}{Threat from\\the front}} \\
      & ConstructionObstacleTwoWays & \\
      & HazardAtSideLaneTwoWays & \\
      & ParkedObstacleTwoWays & \\
      & VehicleOpensDoorTwoWays & \\
      \bottomrule[2pt]
     \end{tabular}
 \end{table}

\subsection{Route Analysis}

The CARLA Leaderboard 2.0 includes 90 routes for training, 2 for development testing, and 20 for validation. Routes in the training and testing sets are sourced from Town 12, while those in the validation set come from Town 13. An important initial question is whether the distribution of scenario types is consistent across these sets. To address this, we counted the number of different scenarios in each route set and visualized their distribution in Fig. \ref{figure: scenario-vs-set}. The training set contains 4,629 scenarios, the development testing set includes 119, and the validation set comprises 1,786. The scenario types exhibit a similar distribution across the sets. Consequently, strong performance on the training set is likely to generalize well to the validation set.

The second issue is that an expert model, even with a 100\% route completion rate and a high driving score, takes over 30 minutes to complete a single route. When the expert agent collects sensory data, the completion time can extend to 3-5 hours, depending on data formats and device performance. By analyzing the distribution of scenarios and weather types across the training set routes (see Fig. \ref{figure: scenario-vs-route}, \ref{figure: weather-vs-route}), we observed that routes 0-29, 30-59, and 60-89 are repeated under different weather conditions. To optimize training efficiency, we propose randomizing the weather types and using only the first 30 routes for data collection during pretraining and online training.

\subsection{Evaluation Metrics}

The CARLA Leaderboards employ three key metrics to assess model performance: route completion, infraction penalty, and driving score. Route completion measures the average ratio of successfully completed routes. Infraction penalty reflects adherence to traffic regulations, diminishing by a percentage when the agent commits infractions or violates traffic rules. The driving score is derived from the product of the route completion ratio and infraction penalty. It offers a comprehensive evaluation of the agent's efficiency and safety. The detailed infraction items are defined and automatically obtained by the CARLA leaderboards, including

\begin{itemize}
    \item collision with pedestrians (\textit{Collisions pedestrians})
    \item collision with other vehicles (\textit{Collisions vehicles})
    \item collision with static elements (\textit{Collisions layout})
    \item running a \textit{Red light}
    \item running a \textit{Stop sign}
    \item driving \textit{Off-road}
    \item agent taking no action for a long time (\textit{Agent blocked})
    \item failure to \textit{Yield to emergency} vehicle
    \item failure to maintain \textit{Minimum speed}
    \item failure to pass a scenario in time (\textit{Scenario timeouts}) - This metric is only available in Leaderboard 2.0 because ``scenario'' is defined before.
    \item deviation from the routes for a distance (\textit{Route deviations})
    \item failure to complete a route in time (\textit{Route timeout})
\end{itemize}

\clearpage

\begin{figure*}[htb]
    \centering
    \includegraphics[width=\textwidth]{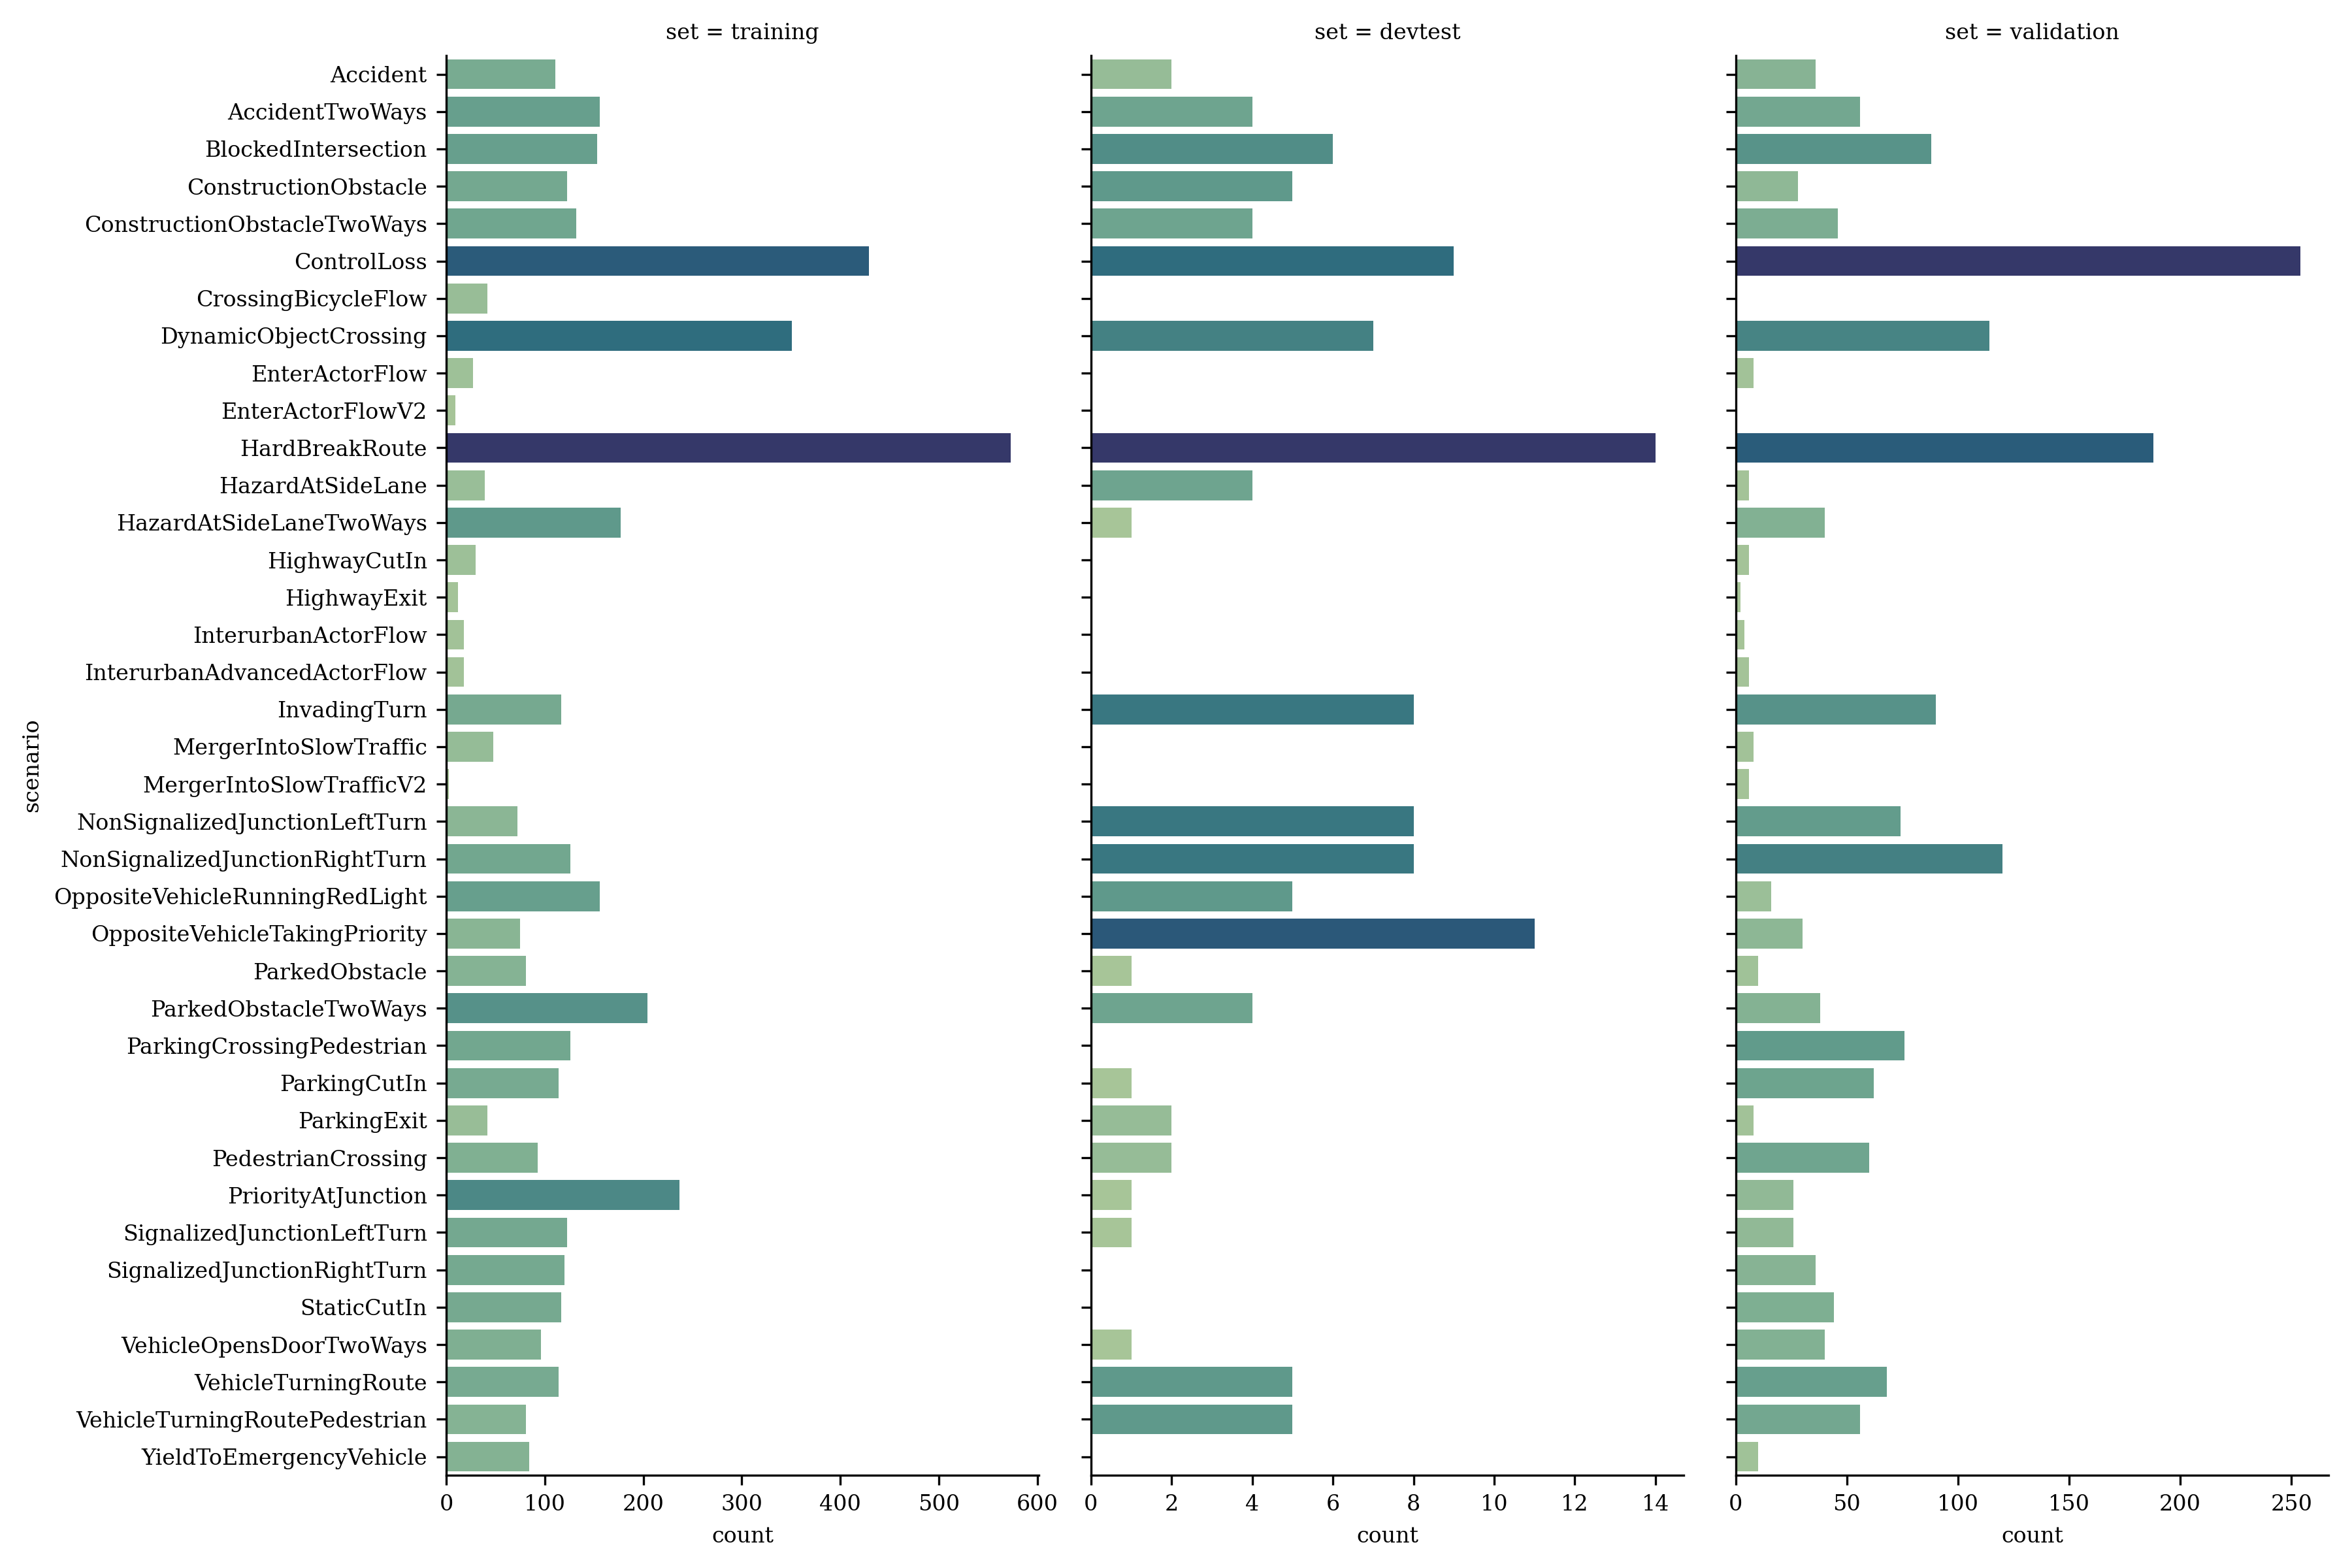}
    \label{figure: scenario-vs-set}
    \caption{Scenario types and their distribution in CARLA Leaderboard 2.0}
\end{figure*}

\begin{figure*}[htb]
    \centering
    \begin{subfigure}
        \centering
        \includegraphics[width=\textwidth]{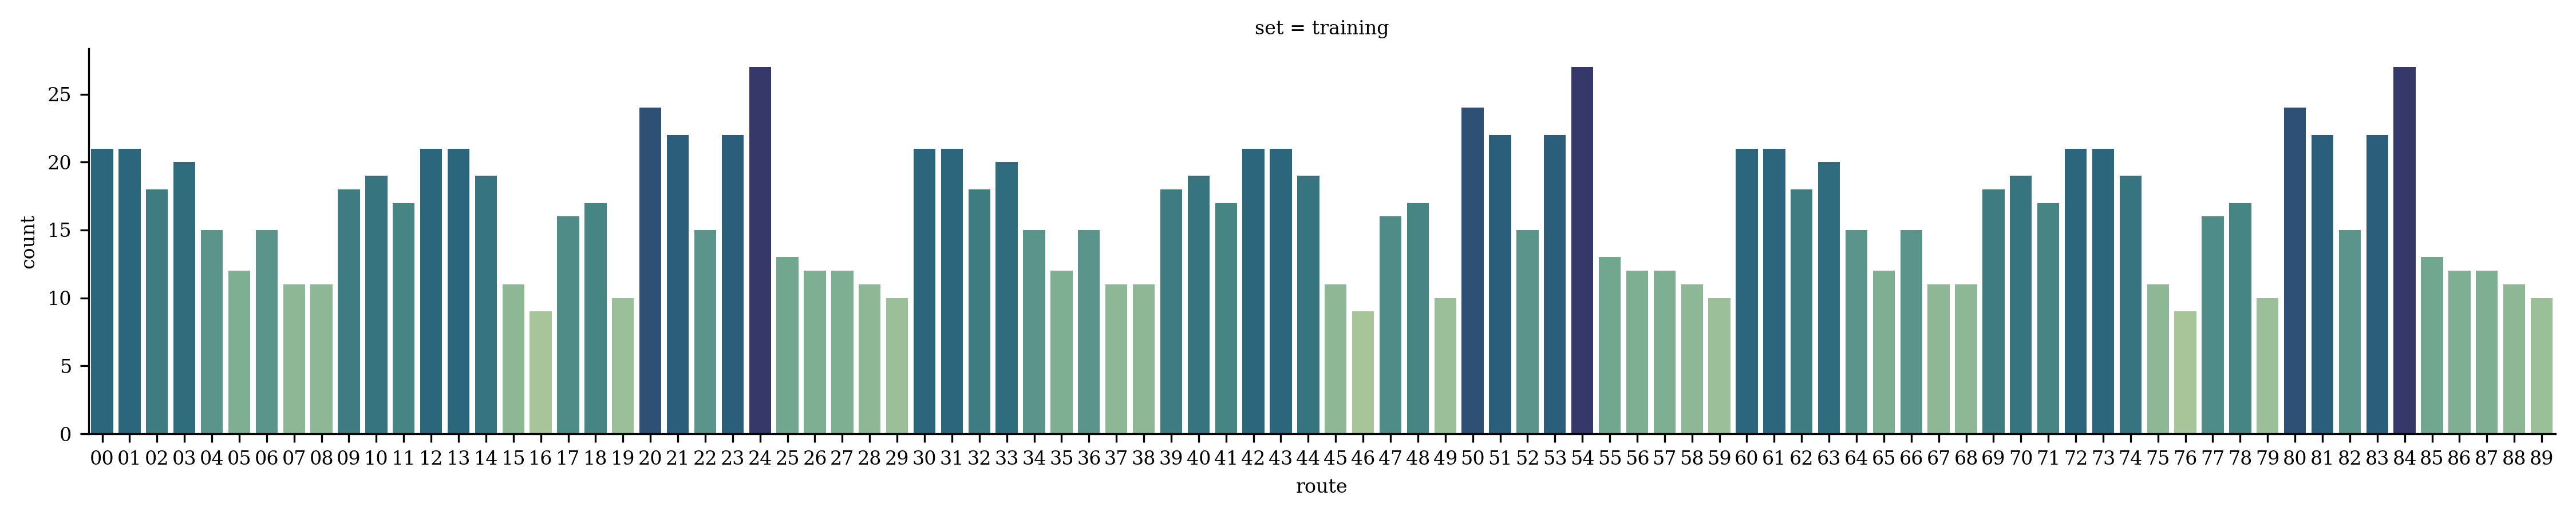}
        \caption{Number of scenarios over routes (Carla Leaderboard 2.0 training set)}
        \label{figure: scenario-vs-route}
    \end{subfigure}
    \begin{subfigure}
        \centering
        \includegraphics[width=\textwidth]{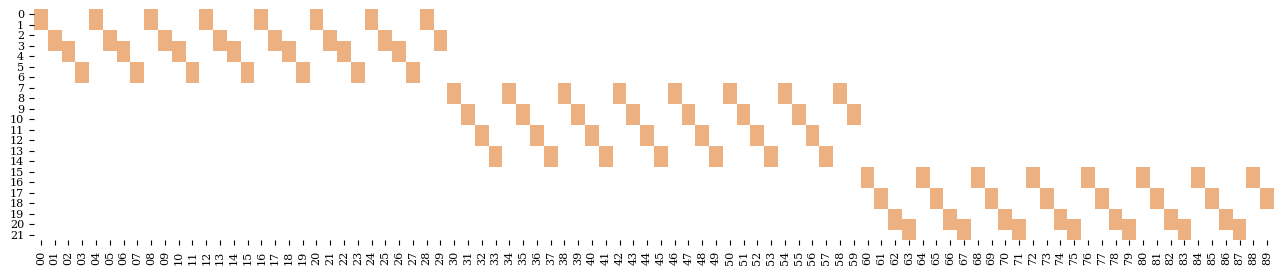}
        \caption{Weather types over routes (Carla Leaderboard 2.0 training set)}
        \label{figure: weather-vs-route}
    \end{subfigure}
\end{figure*}
