# Supplementary material for: From Imitation to Exploration: End-to-end Autonomous Driving based on World Model
Source: arXiv:2410.02253 source file (2025-04-20)
Supplement: Supplementary file 3 [file appendix-model-configuration.tex]

\section{Model Configuration} \label{appendix: model-configuration}

\subsection{Latent Feature Encoder}

\begin{table}[htb]
    \centering
    \caption{Hyper-parameters of SwinTransformer}
    \begin{tabular}{l  l}
        \toprule[2pt]
        \textbf{Hyper-parameter} & \textbf{Value} \\
        \midrule
        Embed dimension & 96 \\
        Depth & [2, 2, 6, 2] \\
        Header number & [3, 6, 12, 24] \\
        Window size & 7 \\
        MLP ratio & 4.0 \\
        QKV bias & True \\
        Hidden dropout & 0.0 \\
        Attention dropout & 0.0 \\
        Drop path rate & 0.3 \\
        \bottomrule[2pt]
    \end{tabular}
\end{table}

\begin{table}[htb]
    \centering
    \caption{Hyper-parameters of the Feature Pyramid Network}
    \begin{tabular}{l  l}
        \toprule[2pt]
        \textbf{Hyper-parameter} & \textbf{Value} \\
        \midrule
        Input channels & [192, 384, 768] \\
        Output channels & 256 \\
        Normalization & BatchNorm2d \\
        \bottomrule[2pt]
    \end{tabular}
\end{table}

\begin{table}
    \centering
    \caption{Hyper-parameters of the PointPillars Encoder (Point Feature Network)}
    \begin{tabular}{l  l}
        \toprule[2pt]
        \textbf{Hyper-parameter} & \textbf{Value} \\
        \midrule
        Input channels & 3 \\
        Feature channels & [128, 128] \\
        Normalization & True \\
        \bottomrule[2pt]
    \end{tabular}
\end{table}

\begin{table}
    \centering
    \caption{Hyper-parameters of the PointPillars Encoder (Scatter Network)}
    \begin{tabular}{l  l}
        \toprule[2pt]
        \textbf{Hyper-parameter} & \textbf{Value} \\
        \midrule
        Input channels & 128 \\
        Output shape & [128, 128] \\
        \bottomrule[2pt]
    \end{tabular}
\end{table}

\begin{table}
    \centering
    \caption{Hyper-parameters of the VAE}
    \begin{tabular}{l  l}
        \toprule[2pt]
        \textbf{Hyper-parameter} & \textbf{Value} \\
        \midrule
        Encoder channels & [32, 64, 128, 256] \\
        Decoder channels & [256, 128, 64, 32] \\
        Flatten dimension & [256, 16, 16] \\
        Latent dimension & 1024 \\
        \bottomrule[2pt]
    \end{tabular}
\end{table}

\subsection{Sequence Model}

\begin{table}
    \centering
    \caption{Hyper-parameters of the Transformer}
    \begin{tabular}{l l}
        \toprule[2pt]
        \textbf{Hyper-parameter} & \textbf{Value} \\
        \midrule
        Stochastic dimension & 1024 \\
        Action dimension & 3 \\
        Feature dimension & 1024 \\
        Key dimension & 1024 \\
        Value dimension & 1024 \\
        Hidden dimension & 2048 \\
        Layer number & 2 \\
        Head number & 8 \\
        Max length & 64 \\
        Dropout rate & 0.1 \\
        \bottomrule[2pt]
    \end{tabular}
\end{table}

\begin{table}
    \centering
    \caption{Dimension of the MLP Predictors}
    \begin{tabular}{l l}
        \toprule[2pt]
        \textbf{MLP} & \textbf{Dimension} \\
        \midrule
        Reward predictor & [1024, 1024, 4] \\
        Terminal predictor & [1024, 1024, 1] \\
        Dynamics predictor & [1024, 1024, 1024] \\
        \bottomrule[2pt]
    \end{tabular}
\end{table}

\subsection{Policy Agent}

\begin{table}
    \centering
    \caption{Hyper-parameters of SAC}
    \begin{tabular}{l l}
        \toprule[2pt]
        \textbf{Hyper-parameter} & \textbf{Value} \\
        \midrule
        State dimension & 2068 \\
        Hidden dimension & 1024 \\
        Action dimension & 2 \\
        $\gamma$ & 0.95 \\
        $\tau$ & 0.001 \\
        Learning rate & 0.0001 \\
        Initial temperature & 0.1 \\
        Target entropy & -2.0 \\
        Replay buffer size & 1000000 \\
        Warm-up steps & 10000 \\
        \bottomrule[2pt]
    \end{tabular}
\end{table}
