# Supplementary material for: From Imitation to Exploration: End-to-end Autonomous Driving based on World Model
Source: arXiv:2410.02253 source file (2025-04-20)
Supplement: Supplementary file 4 [file appendix-sensor-configuration.tex]

\section{Sensor configuration} \label{appendix: sensor-configuration}

Considering the constraints of computational resources and real-time requirements, we have optimized our sensor configuration to meet the minimal requirements for environmental perception. The setup includes four RGB cameras strategically positioned to cover the front, left, right, and rear views of the vehicle. Each camera operates at a resolution of $640 \times 480$ and has a field of view (FOV) of $120^\circ$. Additionally, a LiDAR sensor is mounted on the vehicle's roof, providing a $360^\circ$ scan. This sensor captures approximately 31,000 points across 32 channels per frame, with a detection range of up to 50 meters and a scanning frequency of 10 Hz.

The placement of each sensor is detailed in Table \ref{table: sensor-configuration}, with coordinates referenced from the center of the ego vehicle. Figure \ref{figure: sensor-location} illustrates the vehicle's perception range: the cameras' range is highlighted in red, while the LiDAR's coverage is shown in blue. Collectively, these sensors provide a comprehensive data set that adequately supports the decision-making processes required for autonomous driving.

\begin{figure*}[b]
    \centering
    \includegraphics[width=0.9\textwidth]{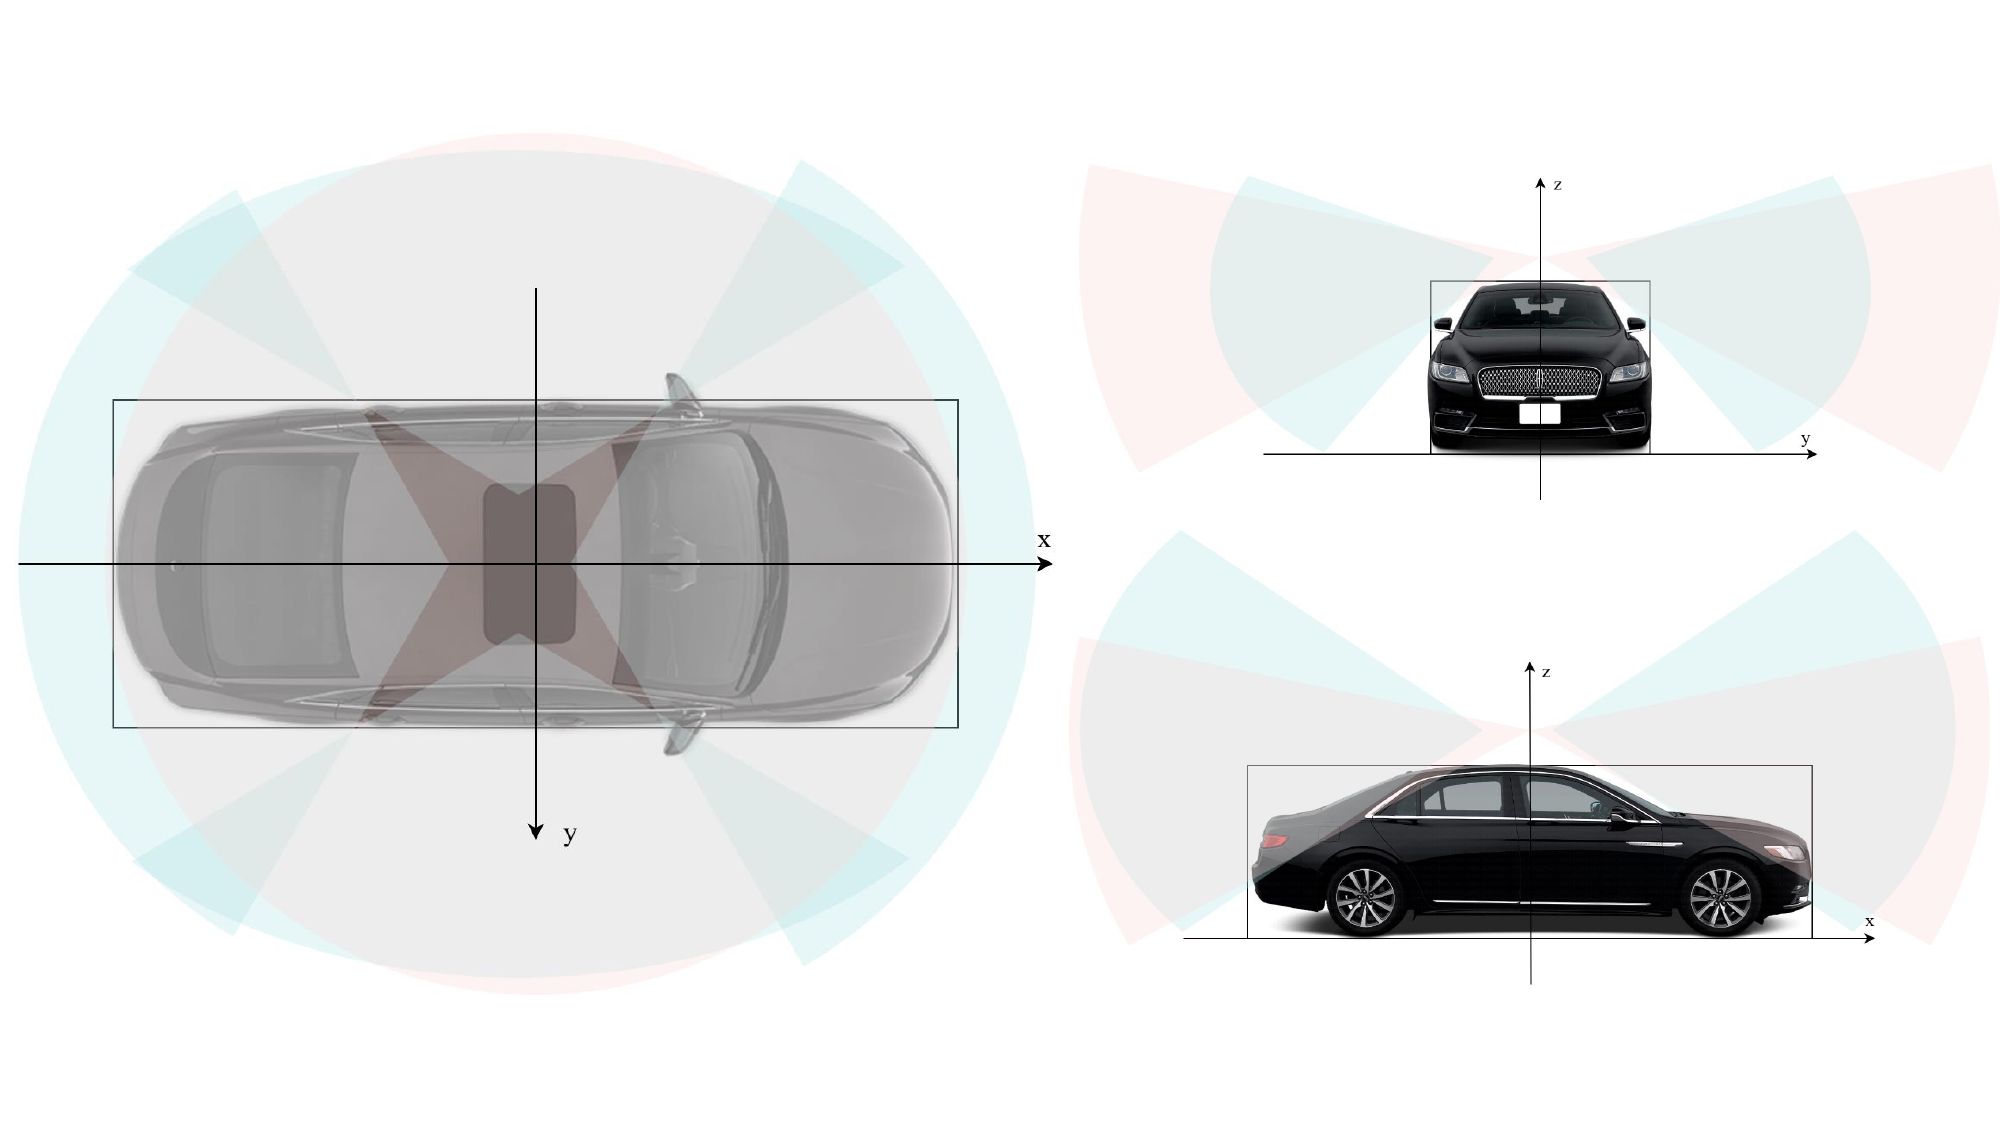}
    \caption{The perception range of the ego vehicle. The cameras' range is highlighted in red, while the LiDAR's coverage is shown in blue}
    \label{figure: sensor-location}
\end{figure*}

\begin{table}[htb]
    \centering
    \caption{The configured sensor's location with respect to the center of the ego vehicle.}
    \label{table: sensor-configuration}
    \begin{tabular}{l|c c c c c c c}
    \toprule[2pt]
        \textbf{Sensor} & x & y & z & roll & pitch & yaw & FOV \\ \midrule
        Camera (front) & 0.2 & 0.0 & 1.8 & 0$^{\circ}$ & 0$^{\circ}$ & 0$^{\circ}$ & 120$^{\circ}$ \\
        Camera (left) & -0.1 & -0.4 & 1.8 & 0$^{\circ}$ & -15$^{\circ}$ & -90$^{\circ}$ & 120$^{\circ}$ \\
        Camera (right) & -0.1 & 0.4 & 1.8 & 0$^{\circ}$ & -15$^{\circ}$ & 90$^{\circ}$ & 120$^{\circ}$ \\
        Camera (rear) & -0.5 & 0.0 & 1.8 & 0$^{\circ}$ & 0$^{\circ}$ & 180$^{\circ}$ & 120$^{\circ}$ \\
        LiDAR & 0.0 & 0.0 & 1.8 & 0$^{\circ}$ & 0$^{\circ}$ & 0$^{\circ}$ & 360$^{\circ}$ \\
        IMU & 0.0 & 0.0 & 0.0 & 0$^{\circ}$ & 0$^{\circ}$ & 0$^{\circ}$ & - \\
        GPS & 0.0 & 0.0 & 0.0 & 0$^{\circ}$ & 0$^{\circ}$ & 0$^{\circ}$ & - \\
        \bottomrule[2pt]
    \end{tabular}
\end{table}
